# Supplementary material for: The Transmission Value of Energy Storage and Fundamental Limitations
Source: arXiv:2407.09428 source file (2024-07-12)
Supplement: Supplementary file 1 [file additional.tex]

%% GMLC case without considering contingency

\subsubsection{Exclusive Transmission Asset Storage} \quad \\
\indent The exclusive case requires the real-time power balance without considering transmission asset storage, where the Unit Commitment (UC) and Economic Dispatch (ED) are solved in advance with infinite transmission line limits based on Prescient \cite{knueven2020novel}, an open source modeling package written in Python for UC and ED optimization.\\
\indent After solving the problem for the peak day, i.e. July 16th, two transmission lines' peak power flow values exceed the given line capacity limits, which is shown in TABLE. \ref{congestline}.
\begin{table}[H]
\caption{The peak line flow and current line capacity of congested lines (Exclusive GMLC)}
\centering
\begin{tabular}{ccc}
\toprule
\textbf{Congested Line} & \textbf{Current Line Capacity} & \textbf{Peak Flow Value} \\ \midrule
C6 (303-309)                          & 175 MW                    & 278.9 MW    \\
CB-1 (318-223)                        & 500 MW                    & 558.4 MW     \\ \bottomrule
\label{congestline}
\end{tabular}
\end{table}
\indent In general, the operators need to re-dispatch some generators to avoid the observed congestion, but if there exists some available transmission asset storage, the operators can directly utilize these transmission assets to enhance the system transmission capability without changing the precious dispatch decisions. TABLE. \ref{storage_current} shows the minimum total transmission asset storage capacity which reduces the original peak flow below the current line capacity limits.
\begin{table}[H]
\caption{The minimum total storage capacity under current line capacity limits (Exclusive GMLC)}
\centering
\begin{tabular}{ccc}
\toprule
\textbf{Storage Location} & \textbf{Storage Capacity} & \textbf{Reduced Line Capacity}\\ \midrule
Bus 223                       & 20.3 MW*4h                & \multirow{3}{*}{162.3 MW}                                                                         \\
Bus 303                       & 82.6 MW*4h                &                                                                                                     \\
Bus 309                       & 62.3 MW*4h                &          \\ \bottomrule                                                \label{storage_current}                                
\end{tabular}
\end{table}
\indent Based on Corollary \ref{totalec}, if the existing line capacity is larger than the peak power flow value, the needed exclusive transmission asset storage is 0. As the line capacity decreases, or the increasing of the peak power flow, more storage should be installed to avoid line overloading. Because there exists the fundamental minimum requirement for the line capacity, i.e. the mean power flow value (Theorem \ref{linecaplim}), Fig. \ref{ex-storage-rts} illustrates that more storage capacity is needed as the transmission line capacity linear proportionally decreases from the peak power flow value to the mean power flow value.\\
\indent Additionally, there exist fundamental limits of transmission line capacity that can be replaced by transmission asset storage (Theorem \ref{theoremcap}). With the fundamental line capacity, the minimum exclusive transmission asset storage capacity is 5546.3 MW$\times$4h, no matter whether based on solving the original optimization problem (\ref{meshedori}) or the reformulated one (\ref{meshedref}) or the closed-form result (\ref{mincap}).
\begin{figure}[H]
\centering
  \includegraphics[scale=0.45]{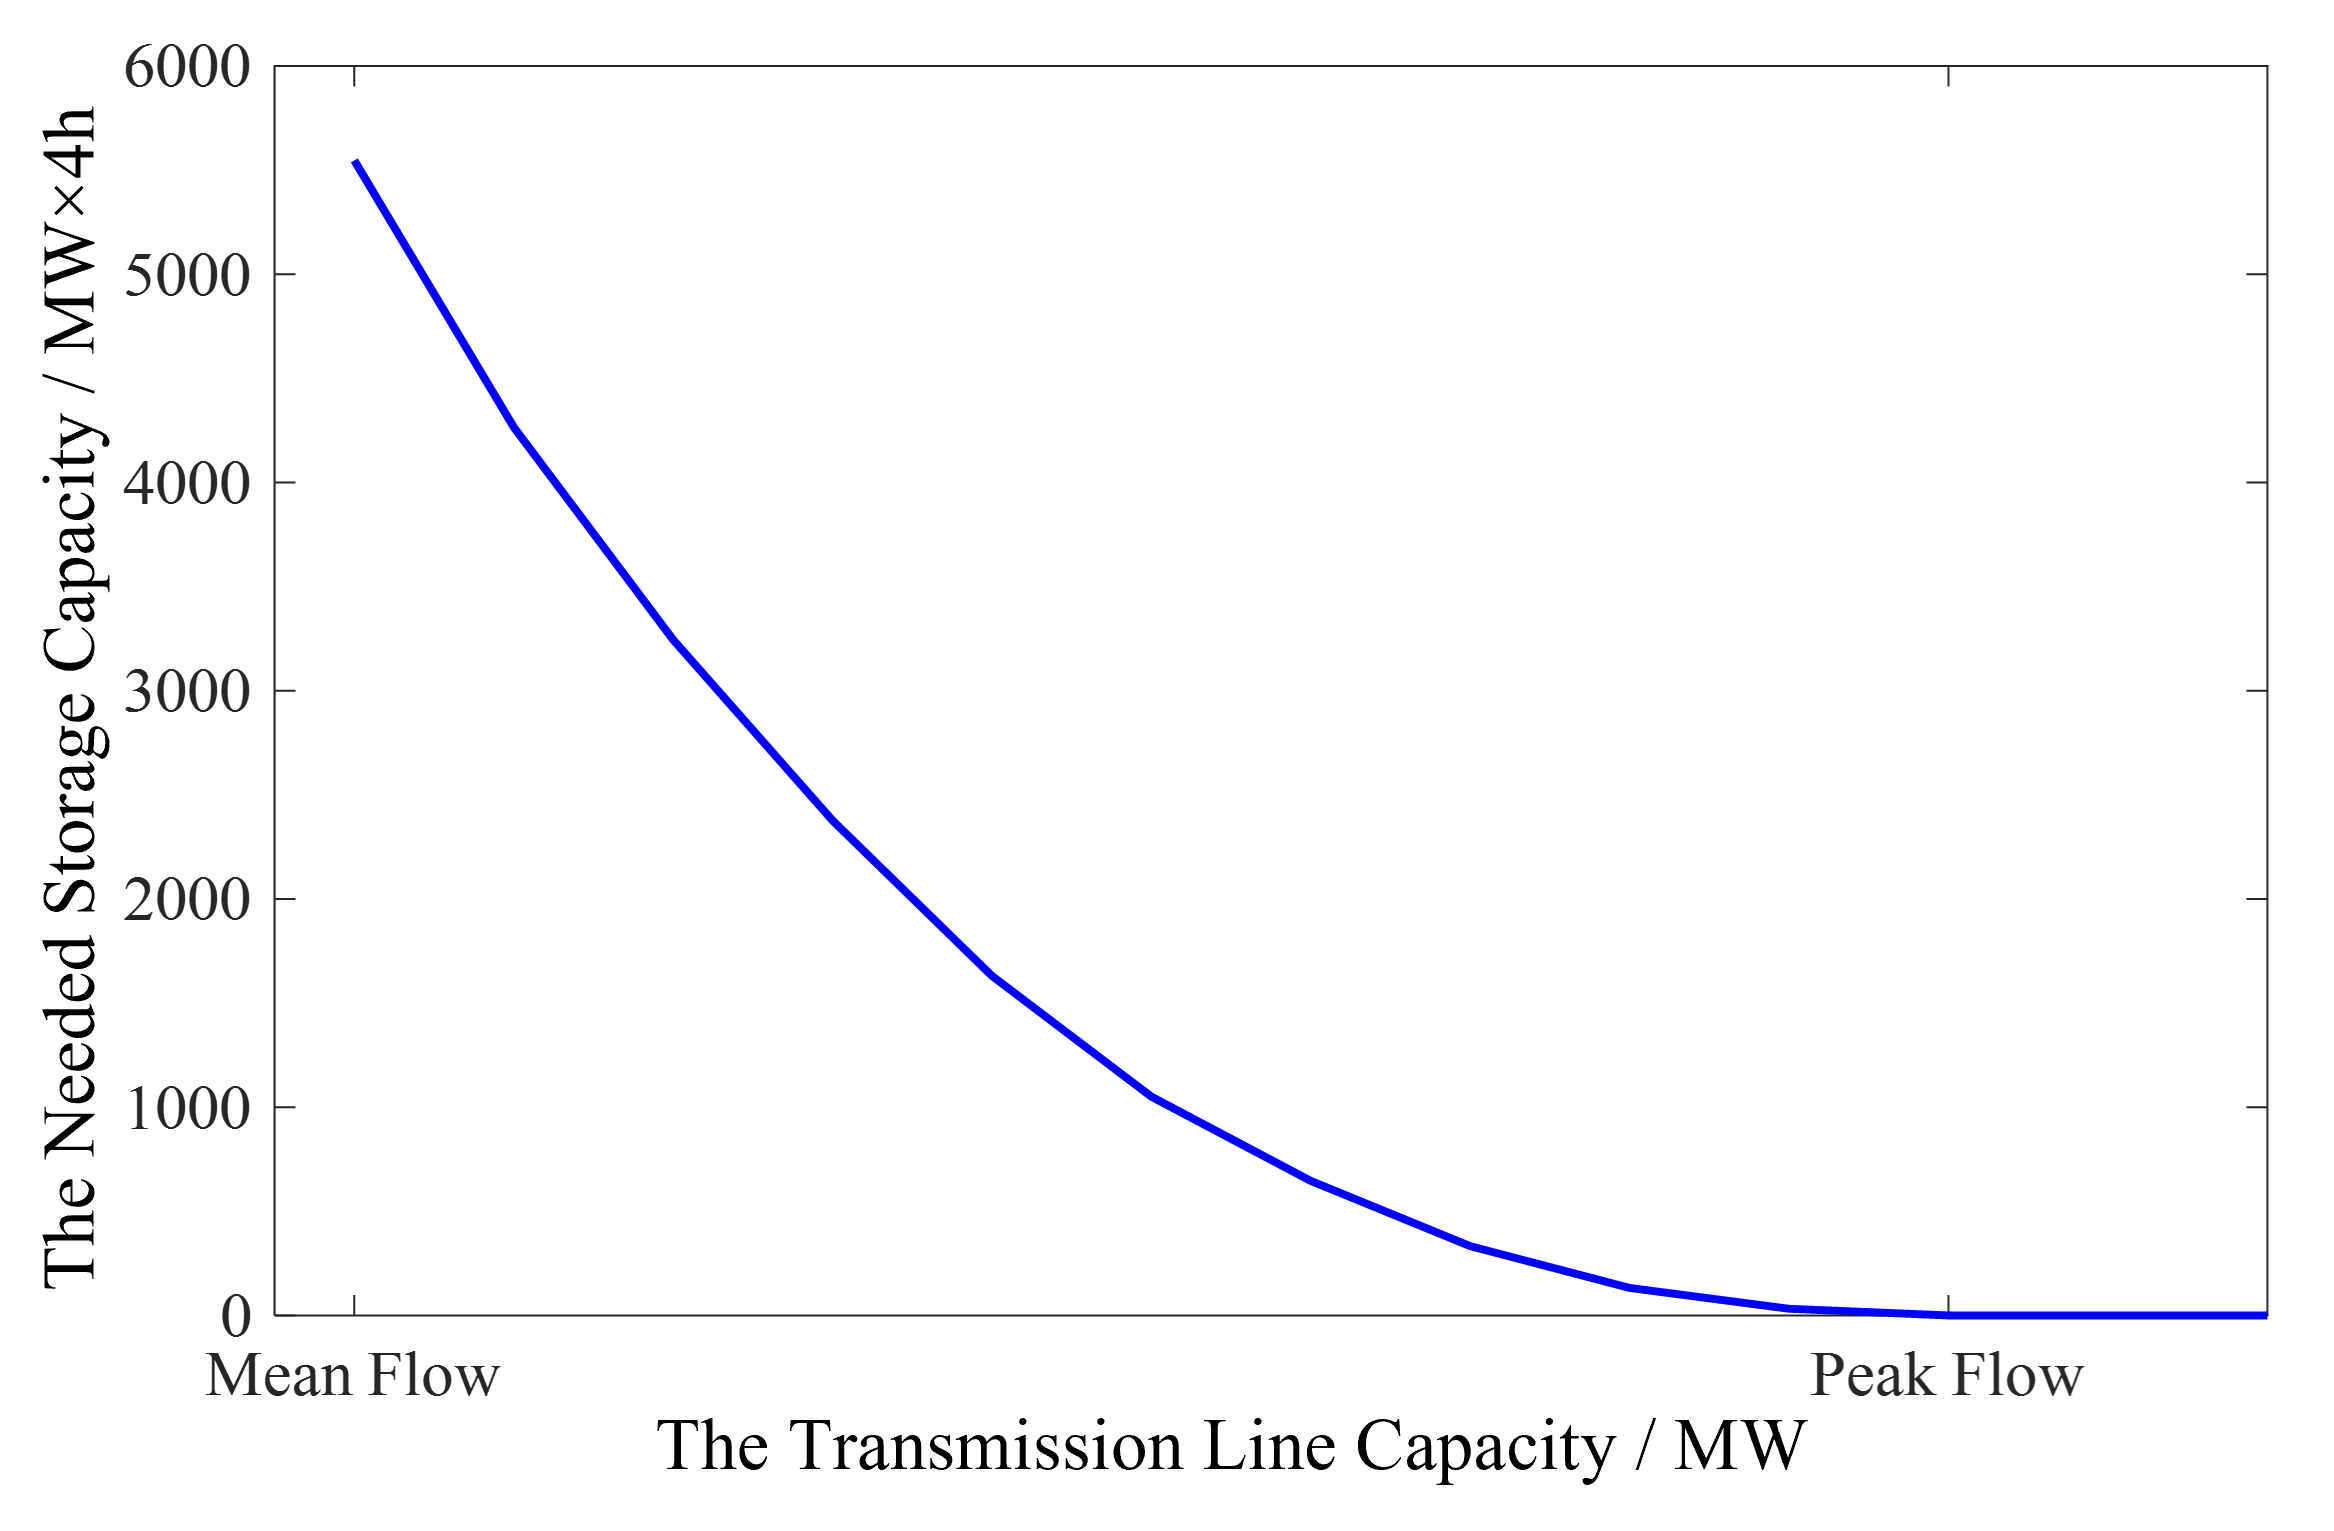}
  \caption{The minimum total storage capacity under different transmission line capacity limits (Exclusive GMLC)}
  \label{ex-storage-rts}
\end{figure}
\subsubsection{Non-Exclusive Transmission Asset Storage}\quad \\
\indent For the non-exclusive case, the transmission asset storage also participates in the real-time power balance work. To better illustrate the dual use of non-exclusive storage, all the dispatchable generators in the original GMLC system are replaced by renewable generators resulting in power imbalances.
\begin{figure}[H]
\centering
  \includegraphics[scale=0.45]{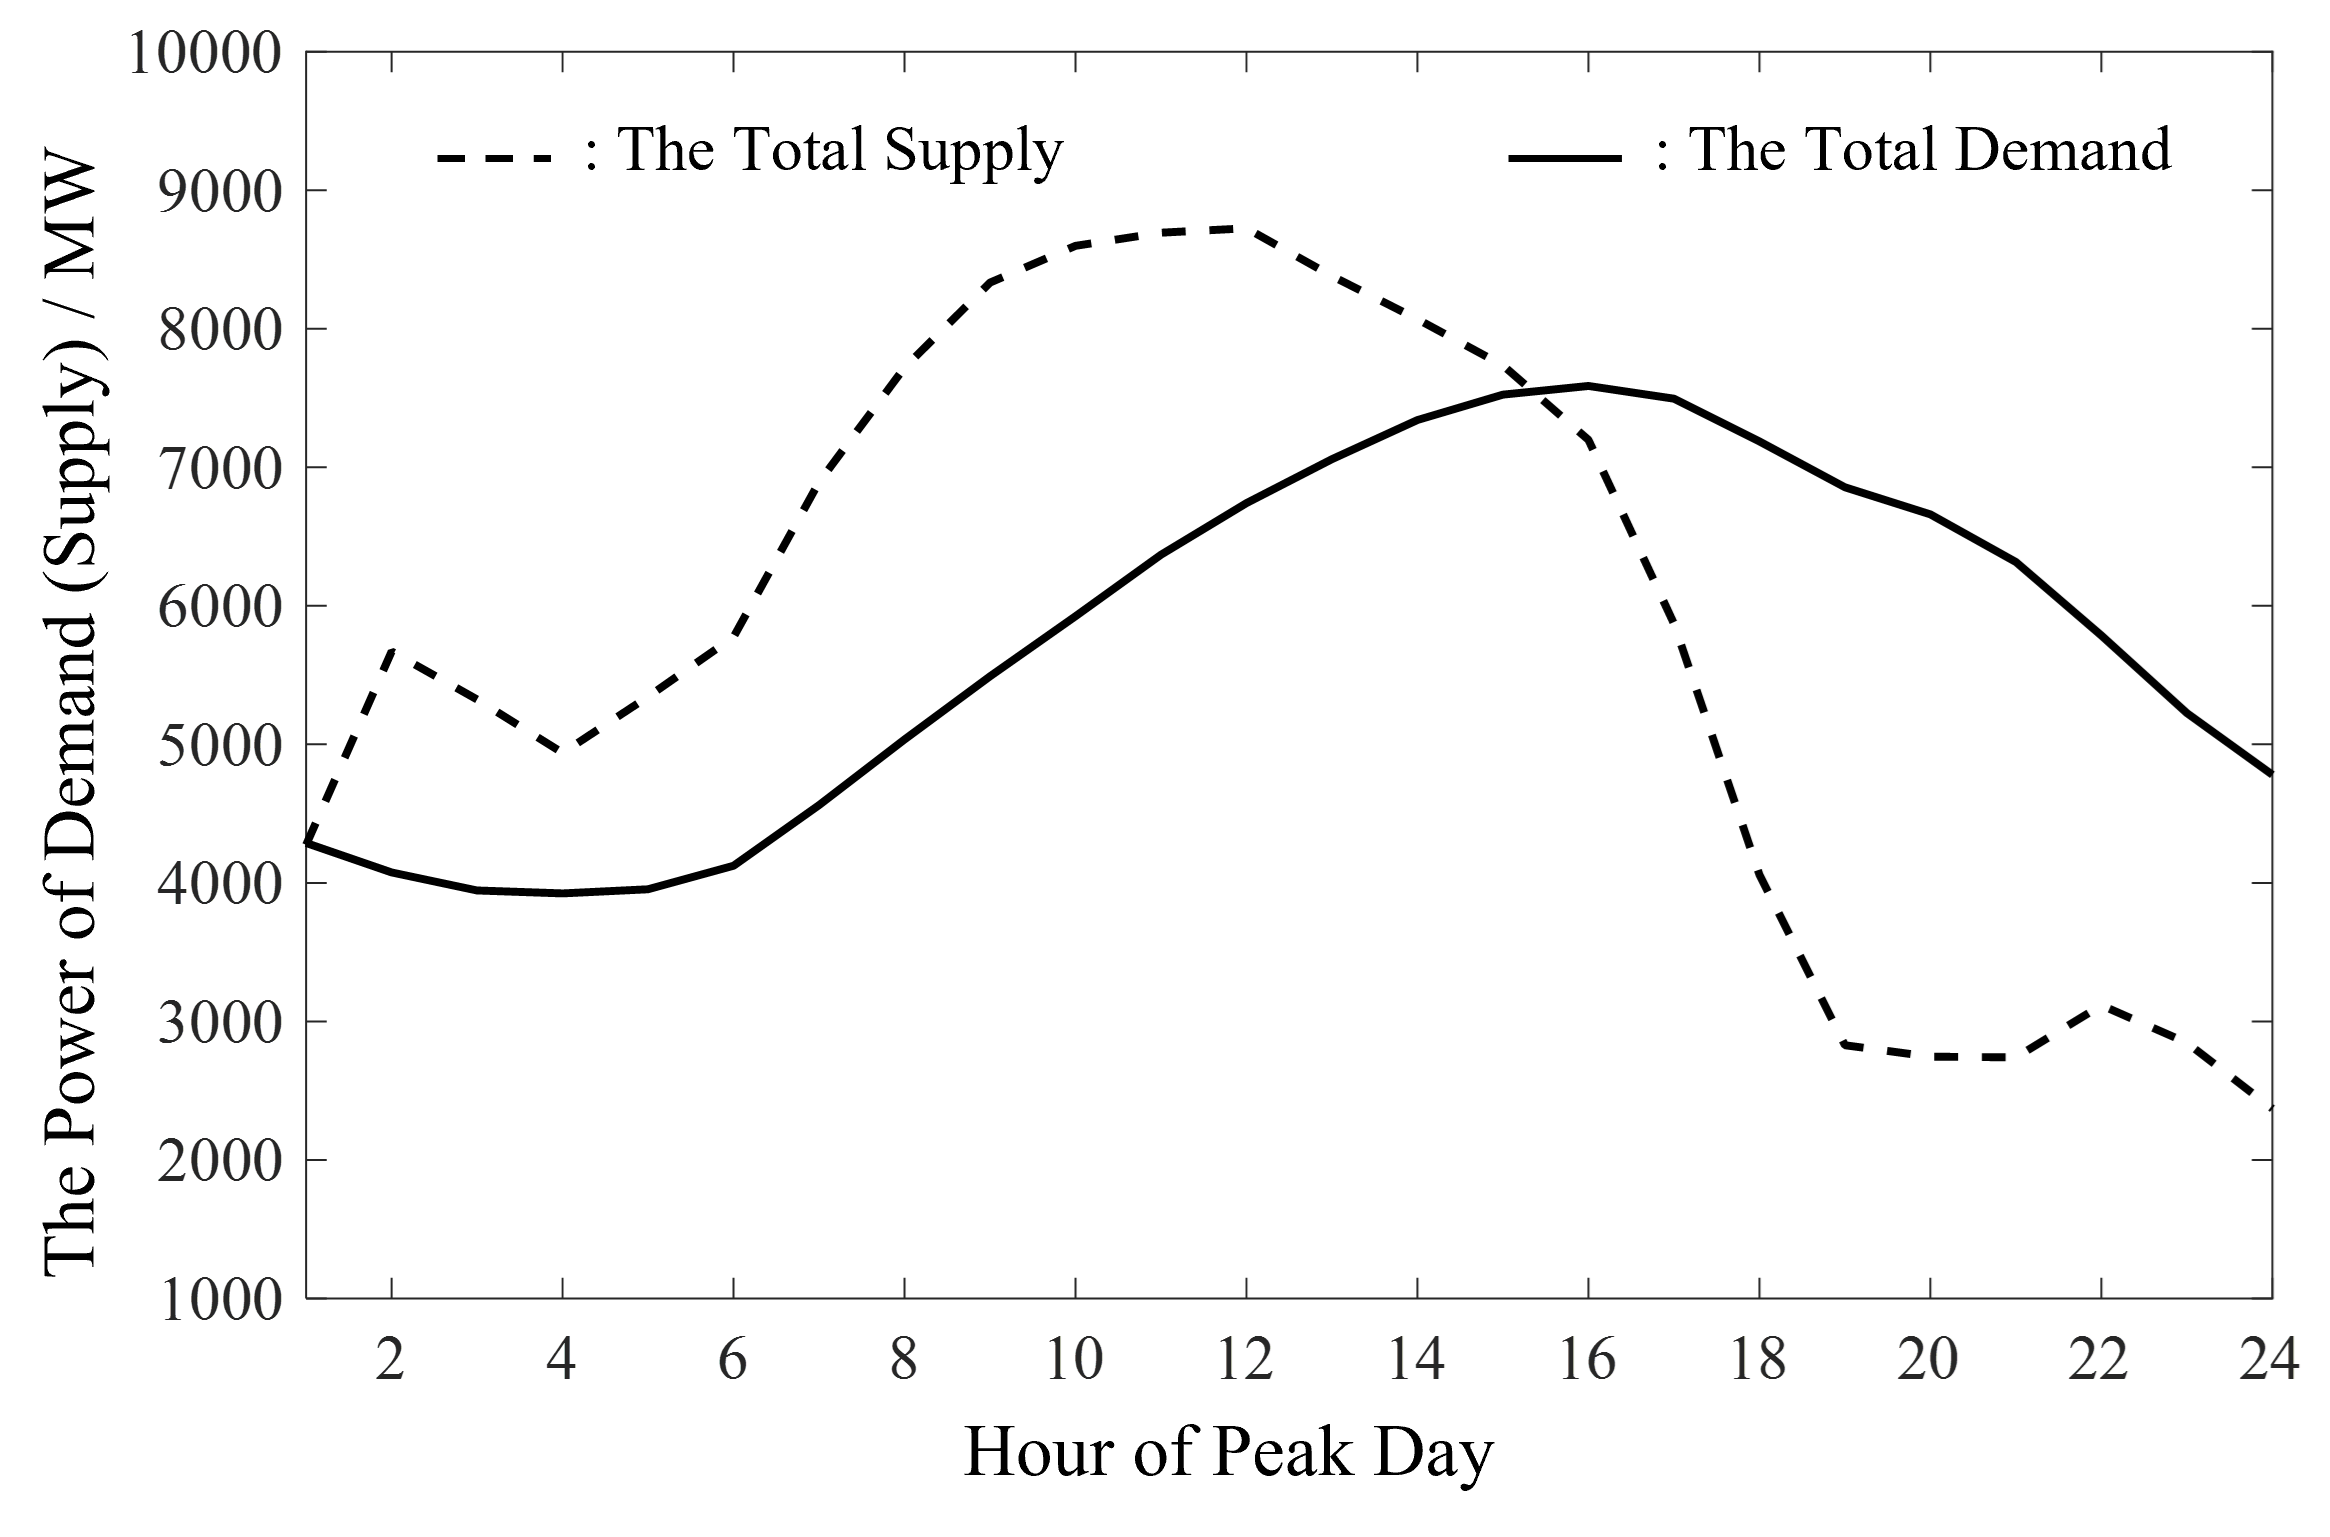}
  \caption{The total supply and demand curve (Non-Exclusive GMLC)}
  \label{non-power-rts}
\end{figure}
\indent Specifically, the power profiles of the previous dispatchable generators are replaced by the total system renewable power curve proportionally, which simulates the 100\% renewable penetration power grids. Because of the storage SoC balance (Assumption \ref{as2}), the total energy generated from all the generators is equal to the total energy consumed from all the loads. The system supply and demand curves are shown in Fig. \ref{non-power-rts}.\\
\indent Similarly, when proportionally linearly tuning the transmission line capacity from mean power flow values to the peak power flow values, the minimum total non-exclusive storage capacity is illustrated in Fig. \ref{non-storage-rts}. The results are the same as proved in Corollary \ref{totalnec}: non-exclusive storage is always needed as long as power imbalances are observed, even if the transmission line capacity is infinite.
\begin{figure}[H]
\centering
  \includegraphics[scale=0.45]{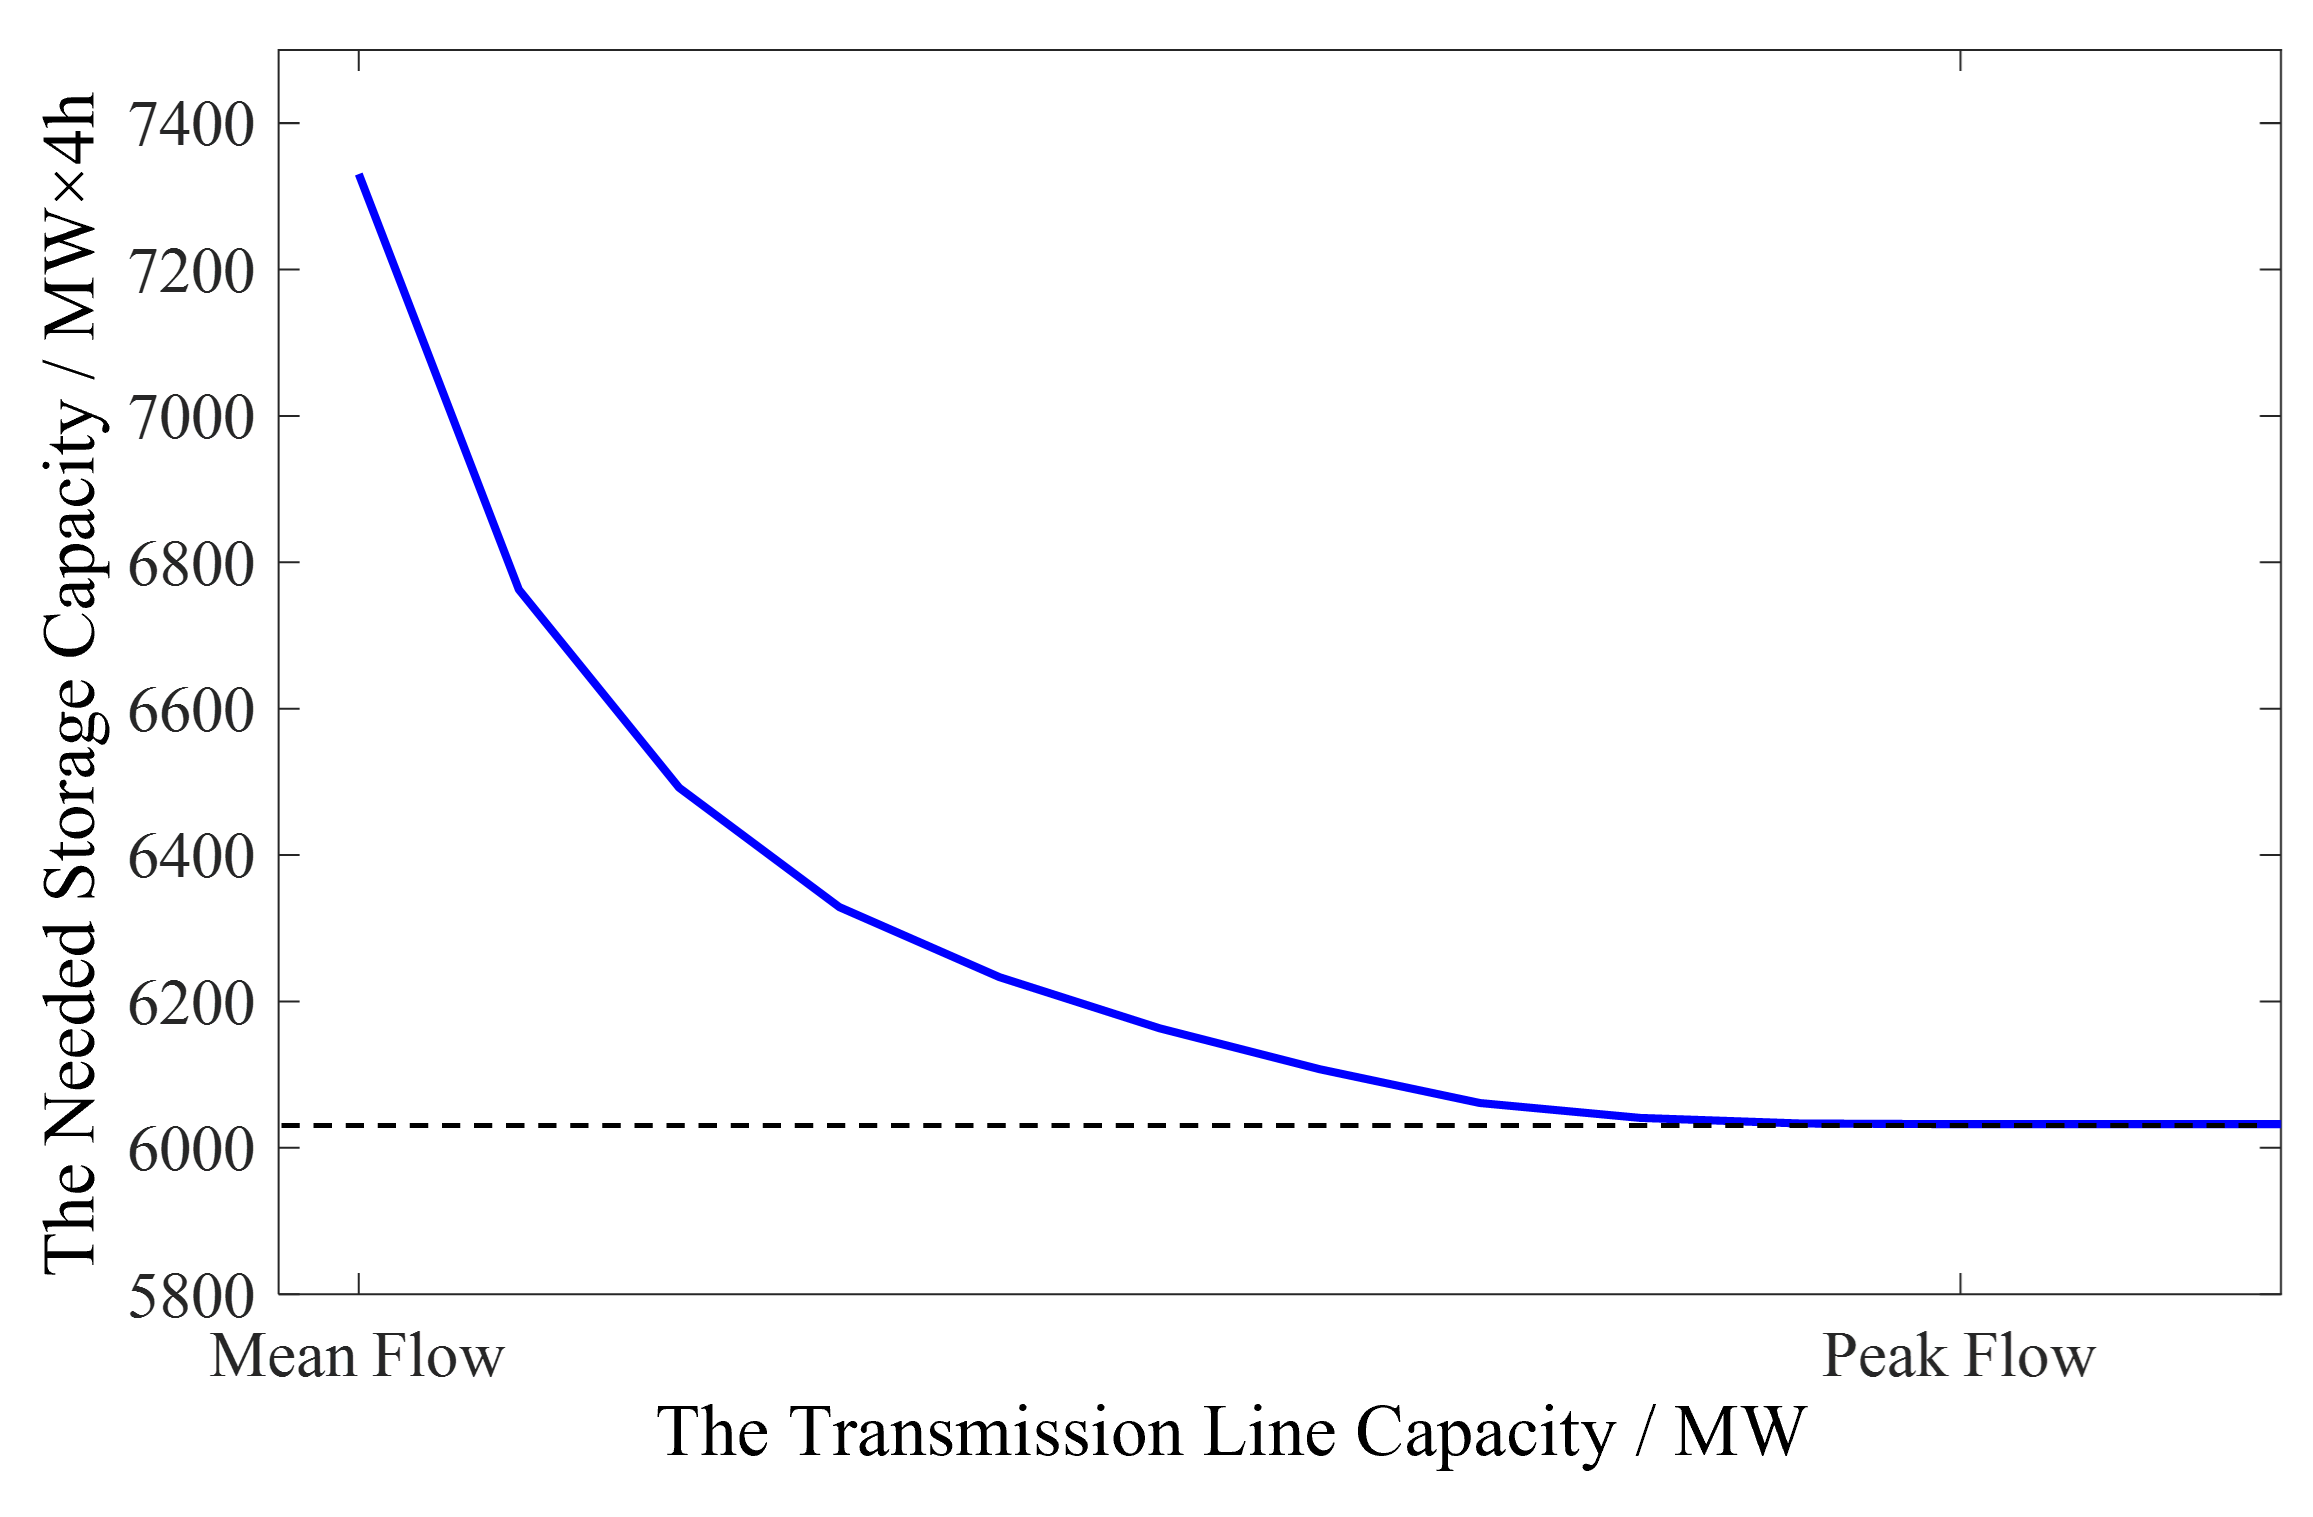}
  \caption{The minimum total storage capacity under different transmission line capacity limits (Non-Exclusive GMLC)}
  \label{non-storage-rts}
\end{figure}
\indent Furthermore, when the line capacity is exactly equal to its fundamental limits, i.e. the mean power flow value, the minimum non-exclusive storage capacity can directly be calculated in closed form (\ref{mincap}), which is 7330.5 MW$\times$4h.

%% The corollary below is all wrong because the t in \max_t is an all different time for different buses!!!!
\begin{corollary}[The Total Exclusive Storage Capacity] \label{totalec}
The total storage capacity is the sum of storage capacity at each bus $i$ can be expressed as:
\begin{equation} \label{mincap}
\min \sum_{i\in \mathcal{N}}X_i = \max_{t \in \mathcal{T}}(\sum_{i\in \mathcal{N}}\widehat{E}'_{i}[t]) - \min_{t \in \mathcal{T}}(\sum_{i\in \mathcal{N}}\widehat{E}'_{i}[t]).   
\end{equation}
Especially, if the capacity of each transmission line is larger than the minimum original line capability, i.e. $\max_{t \in \mathcal{T}}F'_{ij}[t]$, there is \emph{no} need for transmission asset storage, i.e. 
\begin{equation} \label{total0}
\min \sum_{i\in \mathcal{N}}X_i = 0.    
\end{equation}
\begin{proof}
Based on the results of Theorem \ref{theoremcap}, the minimum total storage capacity can be written as:
\begin{equation}
\min \sum_{i\in \mathcal{N}}X_i = \sum_{i\in \mathcal{N}}\{\max_{t \in \mathcal{T}}(\widetilde{E}_i[t] - \widehat{E}'_{i}[t]) - \min_{t \in \mathcal{T}}(\widetilde{E}_i[t] - \widehat{E}'_{i}[t])\}.     
\end{equation}    
Considering the fact that $\widetilde{E}_i[t] = \widehat{E}_{i}[t]$ (Proposition \ref{ees}), after expanding $\widehat{E}_i[t]$ from its definition (\ref{d1e}), we have:
\begin{equation} \label{0sum}
\sum_{i\in \mathcal{N}} \widetilde{E}_i[t] = \sum_{i\in \mathcal{N}} \widehat{E}_i[t] = \sum_{i\in \mathcal{N}} \sum_{t_0=1}^{t} P_{i}[t_0] =  \sum_{t_0=1}^{t} \sum_{i\in \mathcal{N}} P_{i}[t_0] = 0
\end{equation}
Because (\ref{0sum}) is true for \emph{any} time $t \in \mathcal{T}$, which means:
\begin{equation}
\begin{aligned}
\min \sum_{i\in \mathcal{N}}X_i &= \sum_{i\in \mathcal{N}}\{\max_{t \in \mathcal{T}}( - \widehat{E}'_{i}[t]) - \min_{t \in \mathcal{T}}( - \widehat{E}'_{i}[t])\} \\
&= \max_{t \in \mathcal{T}}(\sum_{i\in \mathcal{N}}\widehat{E}'_{i}[t]) - \min_{t \in \mathcal{T}}(\sum_{i\in \mathcal{N}}\widehat{E}'_{i}[t]).    
\end{aligned}
\end{equation}   
Furthermore, if the capacity of each transmission line is larger than the minimum original line capability, there is no need to install exclusive storage to reshape the original line flow, which means the transferred cumulative energy is also equal to the transferred cumulative net energy, i.e.
\begin{equation}
\widetilde{E}'_i[t] =  \widetilde{E}_i[t]  
\end{equation}
Then, based on (\ref{proeseq}) from Proposition \ref{proes}, we have:
\begin{equation} 
\begin{aligned}
\min \sum_{i\in \mathcal{N}}X_i &= \max_{t \in \mathcal{T}}(\sum_{i\in \mathcal{N}}\widehat{E}'_{i}[t]) - \min_{t \in \mathcal{T}}(\sum_{i\in \mathcal{N}}\widehat{E}'_{i}[t]) \\
& = \max_{t \in \mathcal{T}}(\sum_{i\in \mathcal{N}}\widetilde{E}'_{i}[t]) - \min_{t \in \mathcal{T}}(\sum_{i\in \mathcal{N}}\widetilde{E}'_{i}[t])\\
& = \max_{t \in \mathcal{T}}(\sum_{i\in \mathcal{N}}\widetilde{E}_{i}[t]) - \min_{t \in \mathcal{T}}(\sum_{i\in \mathcal{N}}\widetilde{E}_{i}[t])\\
&=0.
\end{aligned}
\end{equation}

\end{proof}
\end{corollary}

\begin{corollary}[The Total Non-Exclusive Storage Capacity] \label{totalnec}
Similar to Corollary \ref{totalec}, the total non-exclusive storage capacity can also be expressed as:
\begin{equation} 
\min \sum_{i\in \mathcal{N}}X_i = \max_{t \in \mathcal{T}}(\sum_{i\in \mathcal{N}}\widehat{E}'_{i}[t]) - \min_{t \in \mathcal{T}}(\sum_{i\in \mathcal{N}}\widehat{E}'_{i}[t]).   
\end{equation}
However, even if the capacity of each transmission line is infinite, there is still a need for non-exclusive transmission asset storage, i.e. 
\begin{equation}
\min \sum_{i\in \mathcal{N}}X_i \neq 0.    
\end{equation}
\begin{proof}
Because $\widehat{E}'_{i}[t] = \widetilde{E}'_i[t]$ is true only when $t=T$ for non-exclusive storage scenario, the previous conclusion (\ref{total0}) dose no longer exists.
\end{proof}
\end{corollary}

\begin{table}[H]
\caption{The minimum storage capacity under different transmission line capacity limits (Exclusive Case)}
\centering
\begin{tabular}{cc}
\toprule
\textbf{Line Capacity}             & \textbf{Minimum Total Storage Capacity}  \\ \midrule
\textbf{120.5 MW (Peak Demand)} & 0                 \\
\textbf{110 MW } & 29.4 MW$\cdot$4h                   \\
\textbf{100 MW (Mean Demand)}        & 82.9 MW$\cdot$4h \\ \bottomrule
\label{t1}
\end{tabular}
\end{table}
